# Supplementary material for: Charge separation in donor-C60 complexes with real-time Green's functions: The importance of nonlocal correlations
Source: arXiv:1801.07712 ancillary file (2018-01-23)
Supplement: Supplementary file 1 [file SI_C60.pdf]

# Charge separation in donor-$C_{60}$ complexes with real-time Green's functions: The importance of nonlocal correlations –Supporting Information–

Emil Viñas Boström,*,† Anders Mikkelsen,‡ and Claudio Verdozzi,†
Enrico Perfetto,¶ and Gianluca Stefanucci§,‖

†*Lund University, Department of Physics and European Theoretical Spectroscopy Facility (ETSF), PO Box 118, 221 00 Lund, Sweden*
‡*Lund University, Department of Physics, PO Box 118, 221 00 Lund, Sweden*
¶*Istituto di Struttura della Materia of the National Research Council, Via Salaria Km 29.3, I-00016 Montelibretti, Italy*
§*Dipartimento di Fisica and European Theoretical Spectroscopy Facility (ETSF), Università di Roma Tor Vergata, Via della Ricerca Scientifica 1, 00133 Rome, Italy*
‖*INFN, Sezione di Roma Tor Vergata, Via della Ricerca Scientifica 1, 00133 Rome, Italy*

E-mail: emil.bostrom@teorfys.lu.se

## KBE and the GKBA equation

The main quantity of interest in the NEGF method is the contour ordered Green's function, defined by[1–3]

$$G_{ji}(z,z') = -i\langle \mathcal{T}\left[c_{j\sigma,H}(z)c^{\dagger}_{i\sigma,H}(z')\right]\rangle. \quad (1)$$

Here the expectation value is taken with respect to the grand-canonical ensemble, the arguments $z$ and $z'$ of the Green's function take values on the Keldysh contour $\gamma$, going from $t = -\infty$ to $t = \infty$ and back again, and the contour-ordering operator $\mathcal{T}$ orders operators so that later contour time arguments are to the left. The equation of motion of the Green's function is (in matrix form)

$$\left[i\frac{d}{dz} - h^{\rm HF}(z;x)\right]G(z,z') = \delta(z,z') + \int_\gamma dz_1 \Sigma(z,z_1)G(z_1,z'), \quad (2)$$

with a corresponding equation being satisfied by its adjoint. Here $h^{\rm HF}$ is the single particle Hamiltonian of the system, which depends parametrically on the nuclear position $x$,[4] and all many-body effects are subsumed in the self-energy $\Sigma$. These equations can be decomposed using the Langreth rules[2] into a set of coupled equations known as the Kadanoff-Baym equations[1–3,5–10] (KBE), where the Green's functions depend on real time arguments. Since the Green's function depends on two time arguments the solution of the KBE scale quadratically with time.

In order to compute the expectation value of any time-local one-body operator, it is enough to have complete knowledge of the one-particle density matrix $\rho_{ji}(t) = -iG^{<}_{ji}(t,t)$. From the equation of motion for the lesser Green's function $G^{<}(t,t')$, and its corresponding adjoint equation, the following equation of motion for

the density matrix can be derived:

$$\frac{d}{dt}\rho(t) + i\left[h^{\mathrm{HF}}(t;x),\rho(t)\right] = -\left(I(t) + h.c.\right). \tag{3}$$

This is not a closed equation for $\rho(t)$ since the collision integral

$$I(t) = \int dt' \left[\Sigma^<(t,t')G^A(t',t) + \Sigma^R(t,t')G^<(t',t)\right] \tag{4}$$

contains the unknown functions $G^A$ and $G^<$. In order to close the equation we make the generalized Kadanoff-Baym ansatz[11,12] (GKBA)

$$G^<(t,t') = \rho(t)G^A(t,t') - G^R(t,t')\rho(t'), \tag{5}$$

where the retarded Green's function $G^R(t,t')$ is taken of the form

$$G^R(t,t') = -i\theta(t-t')Te^{-i\int_{t'}^{t} dt_1 h^{\mathrm{qp}}(t_1)}. \tag{6}$$

There are different ways to construct the quasiparticle Hamiltonian $h^{\mathrm{qp}}$; in this work we have chosen $h^{\mathrm{qp}} = h^{\mathrm{HF}}$.

The computational cost of a real-time NEGF+GKBA simulation with a self-energy in the 2B approximation scales like $T^2$ with $T$ the number of time steps. The scaling with the number $N$ of basis functions ranges between $N^2$ and $N^5$ depending on how sparse is the four index Coulomb tensor $v_{ijmn} = \int drdr'\varphi_i^*(\mathbf{r})\varphi_j^*(\mathbf{r}')\varphi_m(\mathbf{r}')\varphi_n(\mathbf{r})/|\mathbf{r}-\mathbf{r}'|$, where the $\varphi_i$'s form a set of single-particle basis functions. In the present work the scaling is $N^3$ since the Coulomb tensor entering the 2B self-energy diagrams is $v_{ijmn} = \delta_{in}\delta_{jm}U_{ij}$ with $i = H, L$ and $j = 1,\ldots,60$.

# HOMO-LUMO gap

The HOMO-LUMO gap depends on the D–A interaction strength and on the occupations of the HOMO and LUMO levels. To make the discussion transparent we set the D–A hopping integral $t_{da} = 0$. Then, the occupations $n_H$ and $n_L$ are both good quantum numbers and we can label the ground-state energy of the D–A system as $E_g(n_H,n_L)$. For given $n_H$ and $n_L$ the D–A interaction Hamiltonian acts like an external potential on the acceptor:

$$H_{da} = \sum_i \frac{U_{\mathrm{eff}}}{i}(\hat{n}_i - 1) \tag{7}$$

with $U_{\mathrm{eff}} = U_{Ha}(n_H - 2) + U_{La}n_L$. We define $E_a(U_{\mathrm{eff}})$ as the ground-state energy of the isolated acceptor in the presence of the external potential in Eq. (7).

We briefly revisit the gap closure in equilibrium[13] (for clarity, we consider a 1D acceptor, but the $C_{60}$ case can be treated analogously). The ground-state energy of the charge neutral D–A system, i.e., with $n_H = 2$ and $n_L = 0$ is

$$E_g(2,0) = 2\epsilon_H + E_a(0) \tag{8}$$

since $U_{\mathrm{eff}} = 0$ in this case. To obtain the energy of the interacting LUMO we need to calculate the ground-state energy of the D–A system with one more electron on the LUMO, i.e., $E_g(2,1)$, and then subtract $E_g(2,0)$. Taking into account that $U_{\mathrm{eff}} = U_{La}$ in this case one readily finds

$$E_g(2,1) = 2\epsilon_H + \epsilon_L + 2U_{HL} + E_a(U_{La}). \tag{9}$$

Applying the Hellman-Feynman theorem to the difference $\epsilon_L^{\mathrm{eq}} \equiv E_g(2,1) - E_g(2,0)$ we get

$$\epsilon_L^{\mathrm{eq}} = \epsilon_L + 2U_{HL} + \sum_i \frac{1}{i}\left[\int_0^{U_{La}} n_i(U)dU - U_{La}\right] \tag{10}$$

where $n_i(U)$ is the occupation of the $i$-th carbon in the presence of the external potential in Eq. (7) with $U_{\mathrm{eff}} = U$. Since $n_i(U) < 1$ for $U > 0$ we see that the term in the square brackets is always lesser than zero and therefore the D–A interaction decreases the LUMO energy. With a similar analysis one can show that the D–A interaction increases the HOMO energy and therefore the HOMO-LUMO gap shrinks.

We emphasize that $\epsilon_L^{\mathrm{eq}}$ corresponds to the energy required to *add* an electron on the LUMO in the *equilibrium* system. This is an important quantity in molecular transport as the LUMO often represents the most favourable conducting channel. The energy of interest in a CT

process has a different physical origin. Here we are interested in the energy required to *remove* an electron from the LUMO in the *photoexcited* system. This quantity corresponds to the difference $\epsilon_L^x = E_g(1,1) - E_g(1,0)$. Using again the Hellman-Feynman theorem it is straightforward to find

$$\epsilon_L^x = \epsilon_L + U_{HL} + \sum_i \frac{1}{i}\left[\int_{-U_{Ha}}^{-U_{Ha}+U_{La}} n_i(U)dU - U_{La}\right]. \quad (11)$$

The integral can be split in a contribution where $n_i(U) > 1$ (in the interval $[-U_{Ha}, 0]$) and a contribution where $n_i(U) < 1$ (in the interval $[0, -U_{Ha}+U_{La}]$). Depending on which contribution dominates over the other the D–A interaction can both increase and decrease the LUMO energy. For the physical situation discussed in this paper we found that the term in the square brackets is positive and hence LUMO energy increases.

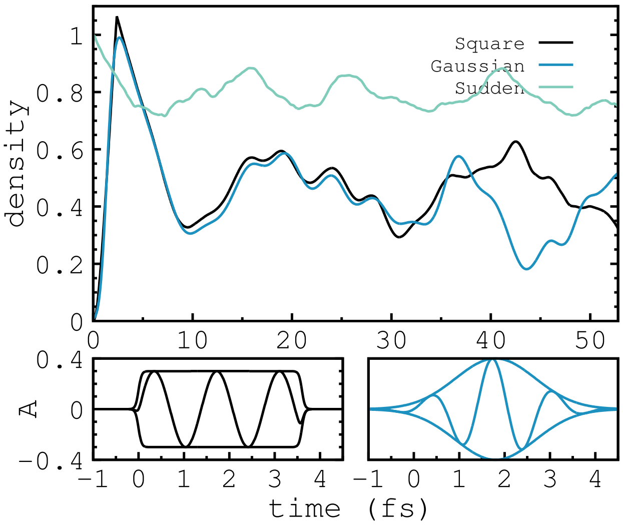


Figure 1: Comparison of time evolution for different excitation protocols, calculated with NEGF. The black curve shows results for a square pulse with amplitude $A = 0.3$ eV and length 2.37 fs (used in the main text), the blue curve for a Gaussian pulse with amplitude $A = 0.4$ eV and FWHM 2.7 fs, and the green for the sudden approximation. All other parameters are as in the main text.

# Initial excitation

In this section we discuss in more detail the initial photoexcitation of the HOMO-LUMO system, and compare the dynamics resulting from different excitations protocols.

We start by considering the excitation field used in the main text. In our simulations the external field is treated in the rotating wave approximation, and is kept on until the LUMO population has reached $n_L \simeq 1$ which happens after approximately for $t = \pi/(3A)$ (a sixth of a Rabi cycle $2\pi/A$). The explicit form of the field is

$$A(t) = Ae^{i\omega t}\left[\theta(t) - \theta(t - t_{\text{off}})\right], \quad (12)$$

where $\theta(t)$ is the Heaviside function and the parameter $t_{\text{off}}$ is adjusted to have $n_L(t_{\text{off}}) \simeq 1$. The resulting pulse consists of a square shaped envelope with a carrier frequency $\omega$, and is illustrated in Figs. 1 and 2.

For comparison we also consider a Gaussian envelope given by the field

$$A(t) = Ae^{i\omega t}e^{-(t-t_{\text{off}}/2)^2/b^2}, \quad (13)$$

where $b$ determines the width of the pulse. The latter is centered around $t = t_{\text{off}}/2$.

In addition we consider the inital state of the sudden approximation, given by $|\Psi^{(1)}\rangle = \frac{1}{2}\sum_\sigma \hat{c}^\dagger_{L\sigma}\hat{c}_{H\sigma}|\Psi_0\rangle$ where $|\Psi_0\rangle$ is the ground state of the system.

In the main text we use the amplitude $A = 0.3$ eV, corresponding to a peak intensity $I = 4.3 \cdot 10^{10}$ W/cm$^2$, that takes a time $t_{\text{off}} = 2.37$ fs to drive an electron from HOMO to LUMO. To obtain similar excitation dynamics with a Gaussian pulse we take $A = 0.4$ eV, corresponding to a peak intensity $I = 5.7 \cdot 10^{10}$ W/cm$^2$, and $b = 1.6$ fs corresponding to a FWHM of 2.7 fs. All other parameters are as in the main text. We show in Fig. 1 the NEGF results for the three different excitations, and in Fig. 2 the resuls for HF. The dynamics following excitation using either of the two real pulses are seen to be in very good qualitative agreement. The situ-

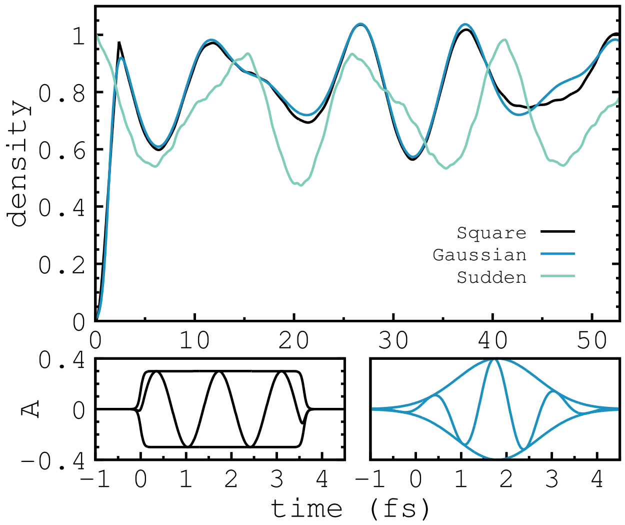


Figure 2: Comparison of time evolution for different excitation protocols, calculated with HF. The black curve shows results for a square pulse with amplitude $A = 0.3$ eV and length 2.37 fs (used in the main text), the blue curve for a Gaussian pulse with amplitude $A = 0.4$ eV and FWHM 2.7 fs, and the green for the sudden approximation. All other parameters are as in the main text.

ation is different for the sudden approximation which gives entirely different results, especially for NEGF as shown in Fig. 1. Similar differences, albeit less marked, are also found in the HFA (see Fig. 2).

## References

(1) Kadanoff, L. P.; Baym, G. *Quantum Statistical Mechanics*; Benjamin, New York, 1962.

(2) Stefanucci, G.; van Leeuwen, R. *Nonequilibrium Many-Body Theory of Quantum Systems*; Cambridge University Press, 2013.

(3) Balzer, K.; Bonitz, M. *Nonequilibrium Green's Functions Approach to Inhomogeneous Systems*; Benjamin, New York, 2013.

(4) Boström, E.; Hopjan, M.; Kartsev, A.; Verdozzi, C.; Almbladh, C.-O. **2016**, *696*, 012007.

(5) Kwong, N.-H.; Bonitz, M. *Phys. Rev. Lett.* **2000**, *84*, 1768–1771.

(6) Dahlen, N. E.; van Leeuwen, R. *Phys. Rev. Lett.* **2007**, *98*, 153004.

(7) Myöhänen, P.; Stan, A.; Stefanucci, G.; van Leeuwen, R. *EPL (Europhysics Letters)* **2008**, *84*, 67001.

(8) Myöhänen, P.; Stan, A.; Stefanucci, G.; van Leeuwen, R. *Phys. Rev. B* **2009**, *80*, 115107.

(9) von Friesen, M. P.; Verdozzi, C.; Almbladh, C.-O. *Phys. Rev. Lett.* **2009**, *103*, 176404.

(10) Hopjan, M.; Verdozzi, C. *First Principles Approaches to Spectroscopic Properties of Complex Materials*; Springer Berlin Heidelberg, 2014; pp 347–384.

(11) Lipavský, P.; Špička, V.; Velický, B. *Phys. Rev. B* **1986**, *34*, 6933–6942.

(12) Haug, H.; Jauho, A.-J. *Quantum Kinetics in Transport and Optics of Semiconductors*; Springer-Verlag, Berlin, 2007.

(13) Myöhänen, P.; Tuovinen, R.; Korhonen, T.; Stefanucci, G.; van Leeuwen, R. *Physical Review B 85, 075105 (2012)* **2012**,
